# Supplementary material for: CeIr$_{3}$Ge$_{7}$: a local moment antiferromagnetic metal with extremely low ordering temperature
Source: arXiv:1804.05131 source file (2018-04-13)
Supplement: Supplementary file 1 [file Supplementary_Material_03282018_ref_update.pdf]

## Supplementary Material for

# $CeIr_3Ge_7$: a local moment antiferromagnetic metal with extremely low ordering temperature

Binod K. Rai[1], Jacintha Banda[2], Macy Stavinoha[3], R. Borth[2], D.-J. Jang[2], Katherine A. Benavides[4], D. A. Sokolov[2], Julia Y. Chan[4], M. Nicklas[2], Manuel Brando[2], C.-L. Huang[1], and E. Morosan[1]

[1]Department of Physics and Astronomy, Rice University, Houston, TX 77005 USA
[2]Max Planck Institute for Chemical Physics of Solids, Dresden, 01187 Germany
[3]Department of Chemistry, Rice University, Houston, TX 77005 USA
[4]Department of Chemistry & Biochemistry, University of Texas at Dallas, Richardson, TX 75080 USA

### Powder and single crystal x-ray diffraction and refinement

Room temperature powder patterns were collected in a Bruker D8 x-ray diffractometer using Cu Kα radiation. The x-ray patterns were refined using TOPAS software. For single crystal x-ray refinement, fragments of $CeIr_3Ge_7$ were obtained by cutting larger crystals to an appropriate size. These fragments were mounted onto glass fibers using epoxy and then mounted onto a Bruker D8 Quest Kappa single crystal x-ray diffractometer equipped with an IμS microfocus source (λ = 0.71073 Å) operating at 50 kV and 1 mA, a HELIOS optics monochromator, and a CMOS detector. The collected data were corrected for absorption using the Bruker program SADABS (multi-scan method). The crystal structure of $CeIr_3Ge_7$ was solved using direct methods in SHELXS2013 [30] and all atomic sites were refined anisotropically using SHELXL2014 [31]. The orientation along the *a* and *c* axes in the hexagonal setting of $CeIr_3Ge_7$ single crystals were determined by the backscattering x-ray Laue method.

Table S1: Crystallographic parameters of $CeIr_3Ge_7$ single crystals at $T$ = 298 K ($R\bar{3}c$)

| Formula | $CeIr_3Ge_7$ |
|---|---|
| $a$ (Å) | 7.8915(8) |
| $c$ (Å) | 20.788(6) |
| $V$ (Å$^3$) | 1121.1(4) |
| Crystal dimensions (mm$^3$) | 0.02x0.04x0.06 |
| $\theta$ range (°) | 5.2-30.3 |
| Extinction coefficient | 0.00102(7) |
| Absorption coefficient (mm$^{-1}$) | 86.73 |
| Measured reflections | 7121 |
| Independent reflections | 384 |
| $R_{int}$ | 0.082 |
| Goodness-of-fit on $F^2$ | 1.18 |
| $R_1(F)$ for $F^2_o>2\sigma(F^2_o)^a$ | 0.032 |

| | |
|---|---|
| $wR_2(F^2_o)^b$ | 0.074 |

$^aR_1 = \sum \| F_o | - | F_c \| / \sum | F_o |$ $^bwR_2 = [\sum[w(F_o^2 - F_c^2)^2] / \sum[w(F_o^2)^2]]^{1/2}$

**Experimental methods**

Temperature-dependent AC resistivity was measured using a Quantum Design (QD) physical properties measurement system (PPMS) with a $^3$He insert using $i$ = 2 mA and $f$ = 622.2 Hz. DC magnetic susceptibility measurements were performed on a QD magnetic properties measurement system equipped with an iHelium $^3$He attachment. Specific heat measurements at ambient pressure were collected using a thermal-relaxation method in QD PPMS with a $^3$He insert for the oriented crystal. An un-oriented crystal is used for the specific heat measurement down to 0.1 K in Dynacool with DR option (Fig. 3(c) in the main text). Specific heat measurements under pressure were performed using a compensated heat-pulse method [34]. The sample was put into a Teflon capsule together with a piece of Pb whose superconducting transition temperature as a function of pressure served as a manometer. The capsule was mounted in a clamped-type CuBe cell using Fluorinert (3M) as a pressure transmitting medium. The background specific heat of the empty cell was determined in separate runs and was subtracted from the raw data to obtain the sample’s contribution.

**Non-Kondo Ce compounds**

Table S2: Non-Kondo Ce compounds. Symbols represent the legend used for Fig. 4 in the main text.

| Compound | Symbol | $T_N$ (K) | Ce-Ce Bond Distance (Å) | References (in the main text) |
|---|---|---|---|---|
| $Ce_3Pt_4$ | ⬗ | 2.8 | 3.514 | 35 |
| CeMgGa | ◒ | 3.1 | 3.897 | 36 |
| CeAuGe | ⬓ | 10.9 | 3.968 | 37 |
| $CePd_2As_2$ | ⬘ | 14.7 | 4.268 | 38 |
| CeAuSn | ▶ | 4.4 | 3.858 | 39, 40 |
| CeAgSn | ◀ | 6.45 | 3.855 | 40 |
| $Ce_2Zn_6Ge_3$ | ⬖ | 7.2 | 4.116 | 41 |
| CeCuSi | ⬒ | 15.5 | 3.977 | 42 |
| CeCuGe | ◑ | 10 | 3.945 | 43 |
| $CeAu_2Ge_2$ | ◧ | 14.5 | 4.367 | 44 |
| $CePd_2In_2$ | ◭ | 4.5 | 4.075 | 45 |
| $CeRu_2Ge_2$ | ▼ | 8.7 | 4.256 | 46 |
| $CeNi_2As_2$ | ◓ | 4.8 | 4.081 | 47 |
| CeCuSn | ◐ | 8.6 | 3.924 | 48 |
| $CeRh_3B_2$ | □ | 115 | 3.096 | 49 |

| | | | | |
|---|---|---|---|---|
| $CeIr_3Si_2$ | ⬙ | 4.1 | 3.607 | 50 |
| $CeRu_2Ga_2B$ | ◨ | 16.3 | 4.187 | 51 |
| CeSbTe | ⧋ | 2.75 | 4.37 | 19 |
| CeSi | ▼ | 5.6 | 3.76 | 52 |
| $CeAg_2Ge_2$ | ⧊ | 4.6 | 4.301 | 53 |
| CeScGe | ▲ | 47 | 3.864 | 54 |
| $CeIr_3Ge_7$ | ★ | 0.63 | 5.724 | current work |
